# Supplementary material for: Intelligent tutoring systems by Bayesian nets with noisy gates
Source: arXiv:2409.04102 source file (2024-09-09)
Supplement: Supplementary file 1 [file 07_appendix.tex]

\clearpage
\appendix
\section{Appendix}

\onecolumn

\begin{center}
\begin{longtable}{c|c|c|c|c|c|c|c|c}
\caption{\textbf{Question skills probabilities}. Q\_ID stays for questions id, Sub\_Q\_ID stays for sub questions id.} \label{tab:bn_topology} \\

\multirow{2}*{\textbf{Q\_ID}}
 & \multirow{2}*{\textbf{Sub\_Q\_ID}}
 & \multicolumn{7}{c}{\textbf{Skills}} \\ 
 ~ & ~ & simple patterns & complex patterns & repetitions & symmetries & voice & prediction & leak  \\ \hline
\endfirsthead

\multicolumn{9}{c}%
{{\tablename\ \thetable{} -- continued from previous page}} \\
\multirow{2}*{\textbf{Q\_ID}}
 & \multirow{2}*{\textbf{Sub\_Q\_ID}}
 & \multicolumn{7}{c}{\textbf{Skills}} \\ 
 ~ & ~ & simple patterns & complex patterns & repetitions & symmetries & voice & prediction & leak  \\\hline 
\endhead

\hline \multicolumn{9}{r}{{Continued on next page}} \\ 
\endfoot

\hline \hline
\endlastfoot

\multirow{6}*{1} 
  & 1 & 0.20 & 0.20 & 0.20 & 0.20 & 0.40 & 0.40 & 0.00 \\ 
~ & 2 & 0.40 & 0.40 & 0.00 & 0.00 & 0.40 & 0.40 & 0.00  \\ 
~ & 3 & 0.20 & 0.20 & 0.20 & 0.20 & 0.20 & 0.20 & 0.00  \\ 
~ & 4 & 0.40 & 0.40 & 0.00 & 0.00 & 0.20 & 0.20 & 0.00  \\ 
~ & 5 & 0.20 & 0.20 & 0.20 & 0.20 & 0.00 & 0.00 & 0.00  \\ 
~ & 6 & 0.40 & 0.40 & 0.00 & 0.00 & 0.00 & 0.00 & 0.00  \\  \hline

\multirow{6}*{2} 
  & 1 & 0.20 & 0.20 & 0.40 & 0.20 & 0.40 & 0.40 & 0.00 \\ 
~ & 2 & 0.40 & 0.40 & 0.00 & 0.00 & 0.40 & 0.40 & 0.00  \\ 
~ & 3 & 0.20 & 0.20 & 0.40 & 0.20 & 0.20 & 0.40 & 0.00  \\ 
~ & 4 & 0.40 & 0.40 & 0.00 & 0.00 & 0.20 & 0.40 & 0.00  \\ 
~ & 5 & 0.20 & 0.20 & 0.40 & 0.20 & 0.00 & 0.00 & 0.00  \\ 
~ & 6 & 0.40 & 0.40 & 0.00 & 0.00 & 0.00 & 0.00 & 0.00  \\  \hline

\multirow{6}*{3} 
  & 1 & 0.70 & 0.00 & 0.90 & 0.20 & 0.70 & 0.70 & 0.20 \\ 
~ & 2 & 0.90 & 0.00 & 0.00 & 0.00 & 0.70 & 0.70 & 0.20  \\ 
~ & 3 & 0.70 & 0.00 & 0.90 & 0.20 & 0.20 & 0.40 & 0.20  \\ 
~ & 4 & 0.90 & 0.00 & 0.00 & 0.00 & 0.20 & 0.40 & 0.20  \\ 
~ & 5 & 0.70 & 0.00 & 0.90 & 0.20 & 0.00 & 0.00 & 0.20  \\ 
~ & 6 & 0.90 & 0.00 & 0.00 & 0.00 & 0.00 & 0.00 & 0.20  \\  \hline

\multirow{6}*{4} 
  & 1 & 0.70 & 0.00 & 0.90 & 0.20 & 0.70 & 0.70 & 0.20 \\ 
~ & 2 & 0.90 & 0.00 & 0.00 & 0.00 & 0.70 & 0.70 & 0.20  \\ 
~ & 3 & 0.70 & 0.00 & 0.90 & 0.20 & 0.20 & 0.40 & 0.20  \\ 
~ & 4 & 0.90 & 0.00 & 0.00 & 0.00 & 0.20 & 0.40 & 0.20  \\ 
~ & 5 & 0.70 & 0.00 & 0.90 & 0.20 & 0.00 & 0.00 & 0.20  \\ 
~ & 6 & 0.90 & 0.00 & 0.00 & 0.00 & 0.00 & 0.00 & 0.20  \\  \hline

\multirow{6}*{5} 
  & 1 & 0.70 & 0.20 & 0.20 & 0.20 & 0.70 & 0.70 & 0.20 \\ 
~ & 2 & 0.90 & 0.40 & 0.00 & 0.00 & 0.70 & 0.70 & 0.20  \\ 
~ & 3 & 0.70 & 0.20 & 0.20 & 0.20 & 0.20 & 0.40 & 0.20  \\ 
~ & 4 & 0.90 & 0.40 & 0.00 & 0.00 & 0.20 & 0.40 & 0.20  \\ 
~ & 5 & 0.70 & 0.20 & 0.20 & 0.20 & 0.00 & 0.00 & 0.20  \\ 
~ & 6 & 0.90 & 0.40 & 0.00 & 0.00 & 0.00 & 0.00 & 0.20  \\  \hline

\multirow{6}*{6} 
  & 1 & 0.20 & 0.70 & 0.20 & 0.00 & 0.90 & 0.70 & 0.20 \\ 
~ & 2 & 0.40 & 0.90 & 0.00 & 0.00 & 0.90 & 0.70 & 0.20  \\ 
~ & 3 & 0.20 & 0.70 & 0.20 & 0.00 & 0.40 & 0.40 & 0.20  \\ 
~ & 4 & 0.40 & 0.90 & 0.00 & 0.00 & 0.40 & 0.40 & 0.20  \\ 
~ & 5 & 0.20 & 0.70 & 0.20 & 0.00 & 0.20 & 0.00 & 0.20  \\ 
~ & 6 & 0.40 & 0.90 & 0.00 & 0.00 & 0.20 & 0.00 & 0.20  \\  \hline

\multirow{6}*{7} 
  & 1 & 0.00 & 0.70 & 0.90 & 0.00 & 0.90 & 0.90 & 0.40 \\ 
~ & 2 & 0.00 & 0.90 & 0.00 & 0.00 & 0.90 & 0.90 & 0.40  \\ 
~ & 3 & 0.00 & 0.70 & 0.90 & 0.00 & 0.40 & 0.70 & 0.40  \\ 
~ & 4 & 0.00 & 0.90 & 0.00 & 0.00 & 0.40 & 0.70 & 0.40  \\ 
~ & 5 & 0.00 & 0.70 & 0.90 & 0.00 & 0.20 & 0.00 & 0.40  \\ 
~ & 6 & 0.00 & 0.90 & 0.00 & 0.00 & 0.20 & 0.00 & 0.40  \\  \hline

\multirow{6}*{8} 
  & 1 & 0.00 & 0.70 & 0.90 & 0.00 & 0.90 & 0.90 & 0.40 \\ 
~ & 2 & 0.00 & 0.90 & 0.00 & 0.00 & 0.90 & 0.90 & 0.40  \\ 
~ & 3 & 0.00 & 0.70 & 0.90 & 0.00 & 0.40 & 0.70 & 0.40  \\ 
~ & 4 & 0.00 & 0.90 & 0.00 & 0.00 & 0.40 & 0.70 & 0.40  \\ 
~ & 5 & 0.00 & 0.70 & 0.90 & 0.00 & 0.20 & 0.00 & 0.40  \\ 
~ & 6 & 0.00 & 0.90 & 0.00 & 0.00 & 0.20 & 0.00 & 0.40  \\  \hline

\multirow{6}*{9} 
  & 1 & 0.00 & 0.90 & 0.90 & 0.00 & 0.90 & 0.90 & 0.40 \\ 
~ & 2 &  &  &  &  &  &  &   \\ 
~ & 3 & 0.00 & 0.90 & 0.90 & 0.00 & 0.40 & 0.70 & 0.40  \\ 
~ & 4 &  &  &  &  &  &  &   \\ 
~ & 5 & 0.00 & 0.90 & 0.90 & 0.00 & 0.20 & 0.00 & 0.40  \\ 
~ & 6 &  &  &  &  &  &  &   \\  \hline

\multirow{6}*{10} 
  & 1 & 0.70 & 0.70 & 0.70 & 0.70 & 0.90 & 0.90 & 0.40 \\ 
~ & 2 & 0.90 & 0.20 & 0.00 & 0.00 & 0.90 & 0.90 & 0.40  \\ 
~ & 3 & 0.70 & 0.70 & 0.70 & 0.70 & 0.40 & 0.70 & 0.40  \\ 
~ & 4 & 0.90 & 0.20 & 0.00 & 0.00 & 0.40 & 0.70 & 0.40  \\ 
~ & 5 & 0.70 & 0.70 & 0.70 & 0.70 & 0.20 & 0.00 & 0.40  \\ 
~ & 6 & 0.90 & 0.20 & 0.00 & 0.00 & 0.20 & 0.00 & 0.40  \\  \hline

\multirow{6}*{11} 
  & 1 & 0.20 & 0.40 & 0.70 & 0.70 & 0.90 & 0.90 & 0.40 \\ 
~ & 2 & 0.40 & 0.70 & 0.00 & 0.00 & 0.90 & 0.90 & 0.40  \\ 
~ & 3 & 0.20 & 0.40 & 0.70 & 0.70 & 0.40 & 0.70 & 0.40  \\ 
~ & 4 & 0.40 & 0.70 & 0.00 & 0.00 & 0.40 & 0.70 & 0.40  \\ 
~ & 5 & 0.20 & 0.40 & 0.70 & 0.70 & 0.20 & 0.00 & 0.40  \\ 
~ & 6 & 0.40 & 0.70 & 0.00 & 0.00 & 0.20 & 0.00 & 0.40  \\  \hline

\multirow{6}*{12} 
  & 1 &  &  &  &  &  &  &  \\ 
~ & 2 & 0.00 & 0.70 & 0.00 & 0.00 & 0.90 & 0.90 & 0.70  \\ 
~ & 3 &  &  &  &  &  &  &   \\ 
~ & 4 & 0.00 & 0.70 & 0.00 & 0.00 & 0.40 & 0.70 & 0.70  \\ 
~ & 5 &  &  &  &  &  &  &   \\ 
~ & 6 & 0.00 & 0.70 & 0.00 & 0.00 & 0.20 & 0.00 & 0.70  \\  \hline
\end{longtable}
\end{center}

\begin{center}
\begin{longtable}{c|c|c|c|c|c|c|c|c|c|c|c|c|c|c|c|c}
\caption{\textbf{Students answers}. Q\_ID stays for questions id, Sub\_Q\_ID stays for sub questions id.} \label{tab:answers} \\

\multirow{2}*{\textbf{Q\_ID}}
 & \multirow{2}*{\textbf{Sub\_Q\_ID}}
 & \multicolumn{15}{c}{\textbf{Student\_ID}} \\ 
 ~ & ~ & 1 & 2 & 3 & 4 & 5 & 6 & 7 & 8 & 9 & 10 & 11 & 12 & 13 & 14 & 15 \\ \hline
\endfirsthead

\multicolumn{17}{c}%
{{\tablename\ \thetable{} -- continued from previous page}} \\
\multirow{2}*{\textbf{Q\_ID}}
 & \multirow{2}*{\textbf{Sub\_Q\_ID}}
 & \multicolumn{15}{c}{\textbf{Student\_ID}} \\ 
 ~ & ~ & 1 & 2 & 3 & 4 & 5 & 6 & 7 & 8 & 9 & 10 & 11 & 12 & 13 & 14 & 15 \\\hline 
\endhead

\hline \multicolumn{17}{r}{{Continued on next page}} \\ 
\endfoot

\hline \hline
\endlastfoot

\multirow{6}*{1} & 1 & no & no & no & yes & no & no & no & no & no & no & yes & no & no & no & no \\ 
~ & 2 & yes & yes & yes & ~ & yes & yes & yes & yes & yes & yes & ~ & no & yes & yes & yes \\ 
~ & 3 & ~ & ~ & ~ & ~ & ~ & ~ & ~ & ~ & ~ & ~ & ~ & no & ~ & ~ & ~ \\ 
~ & 4 & ~ & ~ & ~ & ~ & ~ & ~ & ~ & ~ & ~ & ~ & ~ & no & ~ & ~ & ~ \\ 
~ & 5 & ~ & ~ & ~ & ~ & ~ & ~ & ~ & ~ & ~ & ~ & ~ & no & ~ & ~ & ~ \\ 
~ & 6 & ~ & ~ & ~ & ~ & ~ & ~ & ~ & ~ & ~ & ~ & ~ & no & ~ & ~ & ~ \\ \hline
\multirow{6}*{2} & 1 & no & no & no & no & no & no & no & no & no & no & no & no & yes & no & no \\ 
~ & 2 & yes & yes & yes & no & yes & yes & no & no & yes & yes & yes & yes & ~ & yes & no \\ 
~ & 3 & ~ & ~ & ~ & no & ~ & ~ & no & no & ~ & ~ & ~ & ~ & ~ & ~ & no \\ 
~ & 4 & ~ & ~ & ~ & yes & ~ & ~ & yes & yes & ~ & ~ & ~ & ~ & ~ & ~ & yes \\
~ & 5 & ~ & ~ & ~ & ~ & ~ & ~ & ~ & ~ & ~ & ~ & ~ & ~ & ~ & ~ & ~ \\ 
~ & 6 & ~ & ~ & ~ & ~ & ~ & ~ & ~ & ~ & ~ & ~ & ~ & ~ & ~ & ~ & ~ \\ \hline
\multirow{6}*{3} & 1 & no & no & no & no & no & yes & no & no & no & no & no & no & no & yes & no \\ 
~ & 2 & no & yes & yes & yes & no & no & no & no & no & no & yes & no & yes & ~ & no \\ 
~ & 3 & no & ~ & ~ & ~ & no & ~ & no & no & no & no & ~ & no & ~ & ~ & no \\
~ & 4 & yes & ~ & ~ & ~ & yes & ~ & yes & yes & yes & yes & ~ & no & ~ & ~ & yes \\ 
~ & 5 & ~ & ~ & ~ & ~ & ~ & ~ & ~ & ~ & ~ & ~ & ~ & no & ~ & ~ & ~ \\ 
~ & 6 & ~ & ~ & ~ & ~ & ~ & ~ & ~ & ~ & ~ & ~ & ~ & yes & ~ & ~ & ~ \\ \hline
\multirow{6}*{4} & 1 & no & no & no & no & no & yes & no & no & no & no & no & no & yes & no & no \\ 
~ & 2 & yes & yes & yes & yes & no & ~ & no & no & no & no & yes & no & ~ & yes & yes \\ 
~ & 3 & ~ & ~ & ~ & ~ & no & ~ & no & no & no & no & ~ & no & ~ & ~ & ~ \\ 
~ & 4 & ~ & ~ & ~ & ~ & yes & ~ & yes & yes & yes & yes & ~ & no & ~ & ~ & ~ \\ 
~ & 5 & ~ & ~ & ~ & ~ & ~ & ~ & ~ & ~ & ~ & ~ & ~ & no & ~ & ~ & ~ \\ 
~ & 6 & ~ & ~ & ~ & ~ & ~ & ~ & ~ & ~ & ~ & ~ & ~ & yes & ~ & ~ & ~ \\ \hline
\multirow{6}*{5} & 1 & no & no & no & no & no & no & no & no & no & no & no & no & no & no & no \\ 
~ & 2 & yes & yes & yes & yes & no & yes & no & no & yes & no & yes & no & yes & yes & yes \\ 
~ & 3 & ~ & ~ & ~ & ~ & no & ~ & no & no & ~ & no & ~ & no & ~ & ~ & ~ \\ 
~ & 4 & ~ & ~ & ~ & ~ & yes & ~ & yes & yes & ~ & yes & ~ & yes & ~ & ~ & ~ \\ 
~ & 5 & ~ & ~ & ~ & ~ & ~ & ~ & ~ & ~ & ~ & ~ & ~ & ~ & ~ & ~ & ~ \\ 
~ & 6 & ~ & ~ & ~ & ~ & ~ & ~ & ~ & ~ & ~ & ~ & ~ & ~ & ~ & ~ & ~ \\ \hline
\multirow{6}*{6} & 1 & no & no & no & no & no & no & no & no & no & no & no & no & no & no & no \\ 
~ & 2 & yes & yes & yes & yes & no & yes & no & no & no & no & yes & no & yes & no & yes \\ 
~ & 3 & ~ & ~ & ~ & ~ & no & ~ & no & no & no & no & ~ & no & ~ & no & ~ \\ 
~ & 4 & ~ & ~ & ~ & ~ & yes & ~ & yes & no & yes & yes & ~ & yes & ~ & yes & ~ \\ 
~ & 5 & ~ & ~ & ~ & ~ & ~ & ~ & ~ & no & ~ & ~ & ~ & ~ & ~ & ~ & ~ \\ 
~ & 6 & ~ & ~ & ~ & ~ & ~ & ~ & ~ & no & ~ & ~ & ~ & ~ & ~ & ~ & ~ \\ \hline
\multirow{6}*{7} & 1 & yes & no & yes & no & no & yes & no & no & no & no & no & no & no & yes & no \\ 
~ & 2 & ~ & no & ~ & no & no & ~ & no & no & no & no & no & no & no & ~ & no \\ 
~ & 3 & ~ & no & ~ & yes & no & ~ & no & no & no & no & no & no & no & ~ & yes \\ 
~ & 4 & ~ & no & ~ & ~ & yes & ~ & no & yes & yes & no & no & no & no & ~ & ~ \\ 
~ & 5 & ~ & no & ~ & ~ & ~ & ~ & no & ~ & ~ & no & no & no & no & ~ & ~ \\ 
~ & 6 & ~ & no & ~ & ~ & ~ & ~ & no & ~ & ~ & yes & no & yes & no & ~ & ~ \\ \hline
\multirow{6}*{8} & 1 & no & no & yes & yes & no & yes & no & no & no & no & no & no & no & no & yes \\ 
~ & 2 & no & no & ~ & ~ & no & ~ & no & no & no & no & no & no & no & no & ~ \\ 
~ & 3 & no & no & ~ & ~ & no & ~ & no & no & yes & no & no & no & no & no & ~ \\ 
~ & 4 & no & no & ~ & ~ & yes & ~ & no & no & no & no & no & no & no & yes & ~ \\ 
~ & 5 & no & no & ~ & ~ & ~ & ~ & no & no & ~ & no & yes & no & no & ~ & ~ \\ 
~ & 6 & no & no & ~ & ~ & ~ & ~ & no & no & ~ & yes & ~ & no & no & ~ & ~ \\ \hline
\multirow{6}*{9} & 1 & no & no & yes & yes & no & yes & no & no & no & no & no & no & no & no & yes \\ 
~ & ~ & ~ & ~ & ~ & ~ & ~ & ~ & ~ & ~ & ~ & ~ & ~ & ~ & ~ & ~ & ~ \\ 
~ & 3 & no & no & ~ & ~ & yes & ~ & no & no & yes & yes & yes & no & no & yes & ~ \\ 
~ & ~ & ~ & ~ & ~ & ~ & ~ & ~ & ~ & ~ & ~ & ~ & ~ & ~ & ~ & ~ & ~ \\ 
~ & 5 & no & no & ~ & ~ & ~ & ~ & no & no & ~ & ~ & ~ & no & no & ~ & ~ \\ 
~ & ~ & ~ & ~ & ~ & ~ & ~ & ~ & ~ & ~ & ~ & ~ & ~ & ~ & ~ & ~ & ~ \\ \hline
\multirow{6}*{10} & 1 & no & yes & no & no & no & yes & no & no & yes & no & no & no & no & no & no \\ 
~ & 2 & no & ~ & yes & no & no & ~ & no & no & ~ & no & no & no & no & no & no \\ 
~ & 3 & no & ~ & ~ & no & no & ~ & no & no & ~ & no & no & no & no & yes & no \\ 
~ & 4 & no & ~ & ~ & yes & yes & ~ & yes & no & ~ & no & yes & yes & no & ~ & no \\ 
~ & 5 & no & ~ & ~ & ~ & ~ & ~ & ~ & no & ~ & no & ~ & ~ & no & ~ & yes \\ 
~ & 6 & no & ~ & ~ & ~ & ~ & ~ & ~ & no & ~ & yes & ~ & ~ & no & ~ & ~ \\ \hline
\multirow{6}*{11} & 1 & no & yes & no & no & no & no & no & no & no & no & no & no & no & no & no \\ 
~ & 2 & no & ~ & yes & no & no & yes & no & no & no & no & no & no & no & no & yes \\ 
~ & 3 & no & ~ & ~ & no & no & ~ & yes & no & no & no & no & no & no & no & ~ \\ 
~ & 4 & no & ~ & ~ & yes & yes & ~ & ~ & no & no & yes & yes & yes & no & yes & ~ \\ 
~ & 5 & no & ~ & ~ & ~ & ~ & ~ & ~ & no & no & ~ & ~ & ~ & no & ~ & ~ \\  
~ & 6 & no & ~ & ~ & ~ & ~ & yes & yes & ~ & ~ & ~ & no & ~ & ~ \\ \hline
\multirow{6}*{12} & ~ & ~ & ~ & ~ & ~ & ~ & ~ & ~ & ~ & ~ & ~ & ~ & ~ & ~ & ~ & ~ \\ 
~ & 2 & no & no & no & no & no & yes & no & no & yes & no & no & no & no & no & no \\ 
~ & ~ & ~ & ~ & ~ & ~ & ~ & ~ & ~ & ~ & ~ & ~ & ~ & ~ & ~ & ~ & ~ \\
~ & 4 & no & no & no & no & yes & ~ & no & no & ~ & yes & no & no & no & yes & no \\ 
~ & ~ & ~ & ~ & ~ & ~ & ~ & ~ & ~ & ~ & ~ & ~ & ~ & ~ & ~ & ~ & ~ \\
~ & 6 & no & no & no & no & ~ & ~ & no & yes & ~ & ~ & no & no & no & ~ & no \\ \hline
\end{longtable}
\end{center}
